# Supplementary material for: Homogeneous crystallization in cyclically sheared frictionless grains
Source: arXiv:2008.01920 source file (2020-08-05)
Supplement: Supplementary file 1 [file SI-31-July-HS.pdf]

# Supplemental Material: Homogeneous crystallization in cyclically sheared frictionless grains

Weiwei Jin*,[1] Corey S. O'Hern,[1,2,3] Charles Radin,[4] Mark D. Shattuck**,[5] and Harry L. Swinney[6]

[1]*Department of Mechanical Engineering and Materials Science, Yale University, New Haven, Connecticut 06520, USA*
[2]*Department of Physics, Yale University, New Haven, Connecticut 06520, USA*
[3]*Department of Applied Physics, Yale University, New Haven, Connecticut 06520, USA*
[4]*Department of Mathematics, University of Texas at Austin, Austin, Texas 78712, USA*
[5]*Benjamin Levich Institute and Physics Department, The City College of New York, New York, New York 10031, USA*
[6]*Center for Nonlinear Dynamics and Department of Physics, University of Texas at Austin, Austin, Texas 78712, USA*

In the Supplemental Materials, we provide additional technical details about the discrete element simulations of cyclic shear described in the main text. We include five sections below describing the following topics: 1) the method used for identifying grains in crystalline environments, 2) details of the computational methods (such as the dependence of the results on the spring constant, form of damping force, simulation time step, and relaxation protocol), 3) description of the measurements of the critical cluster size, 4) simulations of cyclic shear in the absence of gravity, and 5) studies that determine the location in the simulation cell of the onset of crystallization.

### A. Identification of crystalline grains

The criteria we use for identifying spheres that are in crystalline environments are those used by Rietz *et al.* [1]. To quantify the degree of positional order during the cyclic shear, we measure the local bond-orientational order parameter for grain $i$,

$$q_6 = \left( \frac{4\pi}{13} \sum_{m=-6}^{6} \left| \sum_{j=1}^{n_i} \frac{A_{ij}}{A_i} Y_{6m}\left(\alpha_j, \psi_j\right) \right|^2 \right)^{\frac{1}{2}}, \tag{S1}$$

where $n_i$ is the number of the neighboring spheres $j$ sharing a Voronoi cell face with the central grain $i$, and $\alpha_j$ and $\psi_j$ are the polar and azimuthal angles of the bond vector connecting grain $i$ and $j$. The spherical harmonics $Y_{6m}$ are weighted by the factor $A_{ij}/A_i$, where $A_{ij}$ is the surface area of the Voronoi cell face shared by spheres $i$ and $j$, and $A_i$ is the total surface area of the Voronoi cell surrounding sphere $i$. The local packing fraction $\phi_{\rm local}$ is defined as the volume of a single sphere divided by the volume of the Voronoi polyhedron it occupies, while the global packing fraction $\phi$ is defined as the total volume of all of the grains divided by the total volume of all of their Voronoi cells.

A sphere is classified as "crystalline" if it is densely packed with the local packing fraction $\phi_{\rm local} > 0.72$ and highly ordered with local bond-orientational order that differs by less than $\pm 0.02$ from the values for perfect FCC (with $q_6(\text{FCC}) = 0.575$) or perfect HCP (with $q_6(\text{HCP}) = 0.485$) order [1].

### B. Computational Methods

In this section, we investigate whether details of the computational methods for simulating cyclic shear affect our results. In particular, we show results for the local and global packing fraction as a function of the magnitude of the spring constant, form of damping force, simulation time step, and energy relaxation protocol, and we demonstrate that our results are largely unaffected by the choices of these parameters.

#### B.1 Spring constant

We are interested in carrying out discrete element simulations of hard grains in the large spring constant limit ($k \to \infty$), where the overlaps between grains tend to zero. However, simulations of hard grains are computationally

costly because the simulation time step required to achieve a given accuracy must become extremely small, $\Delta t \sim \sqrt{m/k}$, where $m$ is the mass of an individual grain. Thus, we chose to simulate systems composed of grains with finite interparticle overlaps and estimate the packing fraction in the limit of hard grains.

We first consider a packing of grains under gravity at $k_0 = 6.54 \times 10^2$ N/m (i.e., $10^4 mg/d$), increase the spring constant of the spheres by roughly a factor of 2, minimize the total potential energy, and continue this process until $k = 10^2 k_0$. In Fig. S1, we show the "uncorrected" global packing fraction

$$\phi_u = \frac{\sum_{i=1}^{N} \pi d^3}{6 \sum_{i=1}^{N} V_{cell,i}}, \tag{S2}$$

where $V_{\text{cell},i}$ is the volume of the Voronoi cell of grain $i$, for six systems as a function of the average interparticle overlap,

$$\langle \delta \rangle = \frac{1}{n_{\text{ovl}}} \sum_{i>j} (d - r_{ij})/d, \tag{S3}$$

where $n_{\text{ovl}}$ is the number of distinct interparticle overlaps. We find that the packing fraction decreases with decreasing overlap (and increasing spring constant), reaching a value that is roughly 2% lower than the value at $k_0 = 6.54 \times 10^2$ N/m in the hard-grain limit.

We can correct the error in the packing fraction for systems with non-zero overlaps, by calculating the volume of the spheres with diameters that are reduced by the amount of the interparticle overlap. Thus, a better estimate of the global packing fraction is

$$\phi = \frac{\sum_{i=1}^{N} \pi d^3 \left(1 - \delta_{\text{max},i}\right)^3}{6 \sum_{i=1}^{N} V_{cell,i}}, \tag{S4}$$

where $\delta_{\text{max},i}$ is the maximum overlap between grain $i$ and its neighbors $j$ and $V_{\text{cell},i}$ is the volume of the Voronoi cell of grain $i$. The estimated global packing fractions (solid symbols) in Fig. S1 show excellent agreement with the packing fractions in the zero-overlap limit. The local packing fraction can be obtained in a similar way, using Eq. (S4) without the sum over $i$.

Thus, in the simulations we set the value of the spring constant to be $k = 6.54 \times 10^2$ N/m and show results for the local and global packing fractions using Eq. (S4) to obtain the value in the zero-overlap limit.

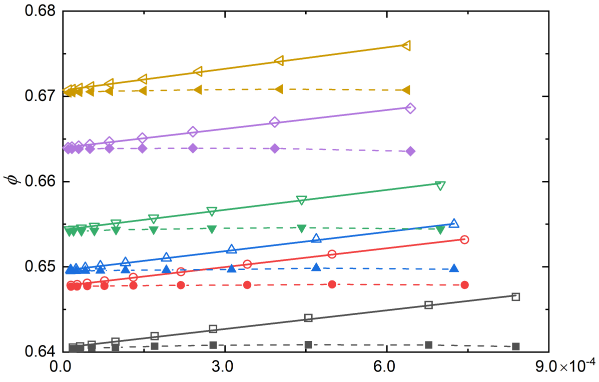


FIG. S1. The global packing fraction $\phi$ plotted as a function of the average interparticle overlap $\delta$. The open symbols, from right to left, correspond to the uncorrected packing fraction for packings generated using spring constants $k/k_0 = 10^0$, $10^{0.25}$, $10^{0.5}$, $10^{0.75}$, $10^1$, $10^{1.25}$, $10^{1.5}$, $10^{1.75}$, and $10^2$. The corresponding solid symbols indicate the packing fraction estimated from Eq. (S4), which takes into account interparticle overlaps.

### B.2. Drag Force

The damping force arises from Stokes drag on particles that interact with the fluid in the shear cell, $F_d \sim (v_i - v_{\text{fluid}})$. We study two forms for the fluid velocity, $v_{\text{fluid}}$. In the first case, we set $v_{\text{fluid}} = 0$. In the second case, the velocity of

the fluid is set to be the same as the velocity of the oscillating cell walls,

$$\vec{v}_{\text{fluid}} = \vec{v}_{\text{cell}} = yA\omega\cos(\omega t)\sec^2(\theta)\hat{x}, \tag{S5}$$

where $y$ is the height from the bottom wall, $A$ is the shear amplitude, $\omega$ is the oscillation frequency, and $\theta$ is the angle that the walls make with the vertical axis. (See Fig. 1(a) in the main text.)

We show the evolution of the global packing fraction versus the number of cycles for the two choices for the fluid velocity in Fig. S2(a). At short times (i.e., for shear cycles $n < 60$), the packing fraction versus cycle number is similar for the two models for $v_{\text{fluid}}$, while for $n > 60$ the results differ. However, in Fig. S2(b), we show that the curves for the percentage of crystalline grains versus packing fraction (over the full range of cycle number) for both models overlap. Thus, the form of the fluid velocity has a negligible influence on the results for the structural properties of the system, like the packing fraction.

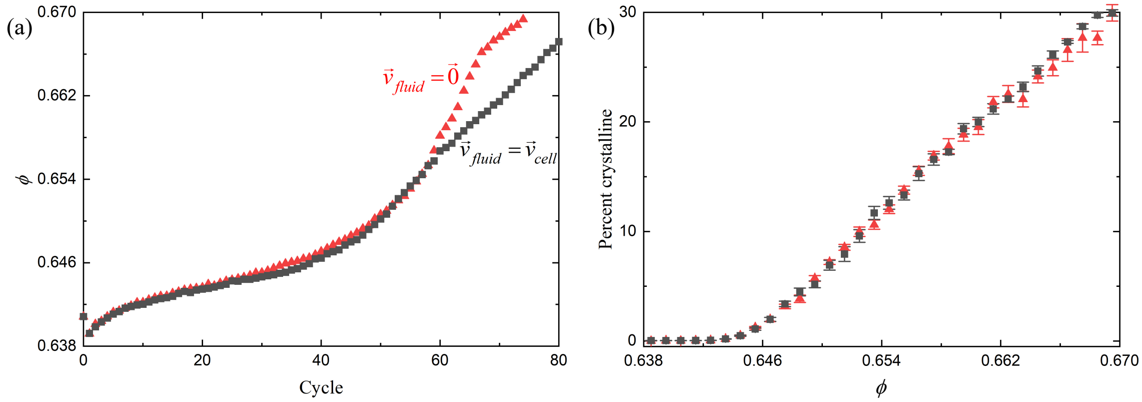


FIG. S2. (a) The global packing fraction $\phi$ plotted as a function of the cycle number $n$ for simulations where the fluid velocity $v_{\text{fluid}} = 0$ (red triangles) or $v_{\text{fluid}}$ is equal to the velocity of the moving cell walls (black squares) at shear amplitude $A = 0.0833$ rad. Each set of data is averaged over six independent simulations. (b) The percentage of grains that are crystalline plotted as a function of the global packing fraction $\phi$ for the simulations in (a).

### B.3. Simulation timestep

For computational efficiency, it is best to carry out the discrete element method simulations at finite values of the time step $\Delta t$, but also ensure that the results do not depend on the value of the time step. In Fig. S3(a), we show a comparison of the global packing fraction versus cycle number for simulations using four different time steps. The packing fraction $\phi$ versus cycle number is similar for the different time steps at small cycle numbers, but then $\phi$ for the simulations at different time steps begins to deviate for $n > 30$. However, in Fig. S3(b), we show that the simulation time step has a negligible influence on the results when the percentage of the system that has crystallized is plotted versus $\phi$. For all of the simulation results in the main text, we use $\Delta t = 4.4 \times 10^{-5}$ s (45600 steps per cycle), which ensures that the average overlap is less than $10^{-3}$ at $k = 6.54 \times 10^2$ N/m.

### B.4. Energy relaxation protocol

For the results shown in the main text, both the strain and dissipation were applied continuously, i.e. the vertical orientation of the side walls was varied continuously according to Eq. (3) in the main text and energy was dissipated via the drag term in the equation of motion. We also considered a more quasistatic protocol mimicking the experiments of Rietz, *et al.*, in which we move the side walls according to the first protocol by a single full cycle, and then move the grains so that the total energy is minimized at fixed wall positions, and repeat this process for a given number of cycles. The energy minimization is carried out for 2 s, which is the same time that it takes the walls to complete a full cycle. In Fig. S4(a), we show a comparison of the global packing fraction versus cycle number for cyclic shear at amplitude $A = 0.05$ rad using the two energy relaxation protocols. As expected, $\phi$ grows more rapidly with cycle number for the more quasistatic protocol. However, the behavior of the percentage of crystalline grains versus $\phi$

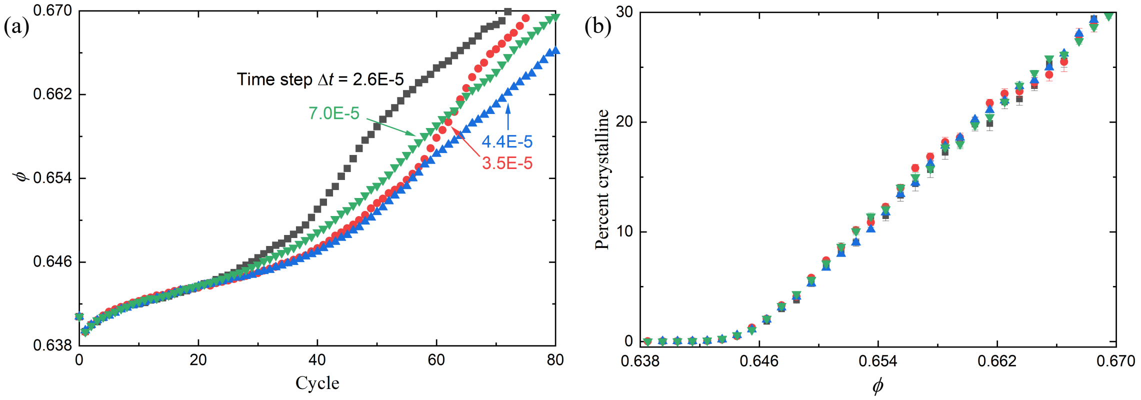


FIG. S3. (a) The global packing fraction $\phi$ plotted as a function of cycle number $n$ for cyclic shear simulations at shear amplitude $A = 0.05$ rad for simulations run with different time steps $\Delta t = 2.6 \times 10^{-5}$ (black squares), $3.5 \times 10^{-5}$ (red circles), $4.4 \times 10^{-5}$ (blue upward triangles), and $7.0 \times 10^{-5}$ s (green downward triangles). (b) The percentage of crystalline grains plotted as a function of the global packing fraction $\phi$ for the simulations in (a). Each curve is averaged over ten independent simulations.

is similar for both energy relaxation protocols. In particular, the percentage of crystalline grains does not begin to increase until $\phi > 0.646$ for both protocols.

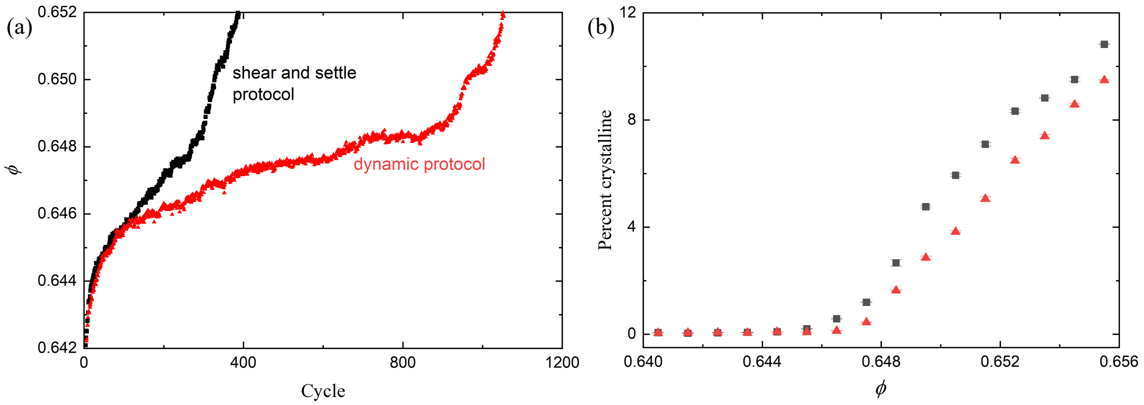


FIG. S4. (a) Global packing packing fraction $\phi$ plotted versus the cycle number during cyclic shear with amplitude $A = 0.05$ rad for the simulations with continuously applied strain dissipation (red triangles) and the quasistatic protocol (black squares). (b) The percentage of crystalline grains plotted as a function of the global packing fraction $\phi$ for the simulations in (a).

### B.5. Setup of shear cell

The model cell used in our simulations differs slightly from the one in the experiment [1]: in the simulations the top of the cell is fixed while bottom oscillates horizontally, and the bottom moves slowly upward as the grains compact, while in the experiment the bottom of the cell oscillates horizontally and its top moves slowly downward as the grains compact. To see if this difference is significant we conducted simulations with the top wall rather than bottom wall moving vertically. Figure S5(a) shows the result for the packing fraction versus cycle number is nearly the same for the two models at small cycle numbers, while for $n > 40$ the results begin to differ. However, in Fig. S5(b), we show that the results for the fraction of the cell that is crystallized as a function of $\phi$ are nearly the same whether the top or bottom wall is allowed to move vertically as the grains compact.

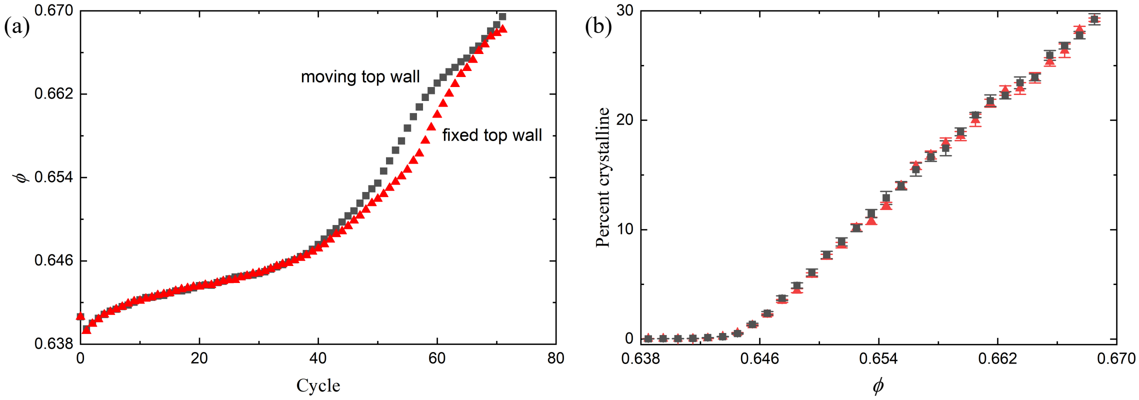


FIG. S5. (a) The global packing fraction $\phi$ plotted as a function of the cycle number $n$ for simulations where the top wall is fixed (red triangles) or the top wall can move vertically (black squares) at shear amplitude $A = 0.0833$ rad. Each set of data is averaged over ten independent simulations. (b) The percentage of grains that are crystalline plotted as a function of the global packing fraction $\phi$ for the simulations in (a).

### C. Critical cluster size

To quantify the critical cluster size during cyclic shear, we measure the probability that a crystallite of a given size will grow $\rho_g$ or shrink $\rho_s$ and determine the crystallite size at which $\Delta\rho = \rho_g - \rho_s > 0$. The probability for a crystallite to grow or shrink is obtained by determining how crystallite sizes evolve after $n_{\rm bin}$ shear cycles. If more than half of the grains forming a given crystallite at the current cycle belong to a larger crystallite after $n_{\rm bin}$ shear cycles, the crystallite is considered to be growing. If more than half of the grains from a given crystallite belong to smaller crystallites after $n_{\rm bin}$ shear cycles, the crystallite is considered to be shrinking. If more than half of the grains forming a crystallite belong to a crystallite with the same size, the crystallite is not counted in the growth or shrinking probability statistics. The value of $n_{\rm bin}$ is chosen to be similar to the cycle number at which the percentage of crystalline grains as a function of $\phi$ begins to deviate from zero in Fig. 4 in the main text. We set $n_{\rm bin} = 1$, 15, 40, and 300 for the simulations at amplitudes $A = 0.1$, 0.0833, 0.0667, and 0.05 rad, respectively.

In Fig. S6(a), we show $\Delta\rho$ for simulations with amplitude $A = 0.05$ rad and the experiments [1] with $A = 0.01$ rad. For both, we find that the critical cluster size is approximately 10 grains. For the simulations with $A = 0.04$, 0.0667, 0.0833, and 0.1, we find critical cluster sizes of $\approx 10$, 13, 16, and 20, respectively, indicating that the critical cluster size approaches 10 in the small-$A$ limit.

In this section, we also discuss two methods for defining the characteristic packing fraction that signals the onset of crystallization. The first definition of the packing fraction at onset is the $\phi$ at which the largest crystallite reaches the critical cluster size (see Fig. S6(b)). Another definition of the packing fraction at the onset of crystallization is the $\phi$ at which the slope of the largest crystallite size in log scale versus packing fraction is the largest. The packing fractions using these two definitions for the onset of crystallization are similar as shown in Fig. S7(a). In the main text, we use the first method for defining the onset of crystallization since it yields smaller values for the standard error.

Note that small crystallites with a size less than the critical cluster size can form before the system reaches the packing fraction at the onset of crystallization. In the experiments, the first packing fraction plateau from shear cycle $n = 20000$ to 70000 in Fig. 1 of the main text does not have any crystallites that are larger than one grain. However, in the experiments, $\phi$ versus cycle number has a second plateau where the small crystallites grow and shrink before reaching the onset of crystallization with crystallites that reach the critical cluster size.

In Fig. S7(b), we plot the global packing fraction at the onset of crystallization (using method 1) as a function of system size. We studied four system sizes containing $N = 5200$, 7900, 11400, and 18200 grains, which corresponds to $N_{\rm inves} = 3335$, 5345, 8055, and 13610 grains that are at least 1.5 diameters from the walls. The packing fraction at the onset of crystallization approaches a well-defined value, $\phi = 0.646 \pm 0.001$, for system sizes with $N_{\rm inves} \gtrsim 8000$.

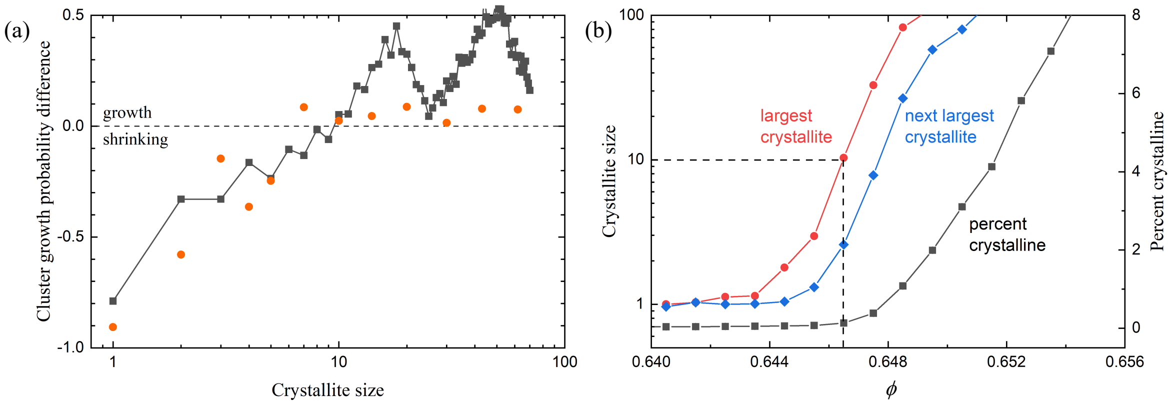


FIG. S6. (a) The difference between the probability that a crystallite will grow versus shrink $\Delta\rho = \rho_g - \rho_s$ during cyclic shear from simulations with amplitude $A = 0.05$ rad (black squares) and from experiments with $A = 0.01$ rad (orange circles). For both the simulations and experiments, the characteristic size of the crystallite at which it begins to grow on average is approximately 10 grains, while smaller crystallites tend to disappear. (b) The largest crystallite (red circles), the next largest crystallite (blue diamonds), and the percentage of crystalline grains (black squares) plotted as a function of the global packing fraction $\phi$ for simulations of cyclic shear at amplitude $A = 0.05$ rad with $N = 18200$ grains. The data was averaged over 10 simulations with different initial conditions.

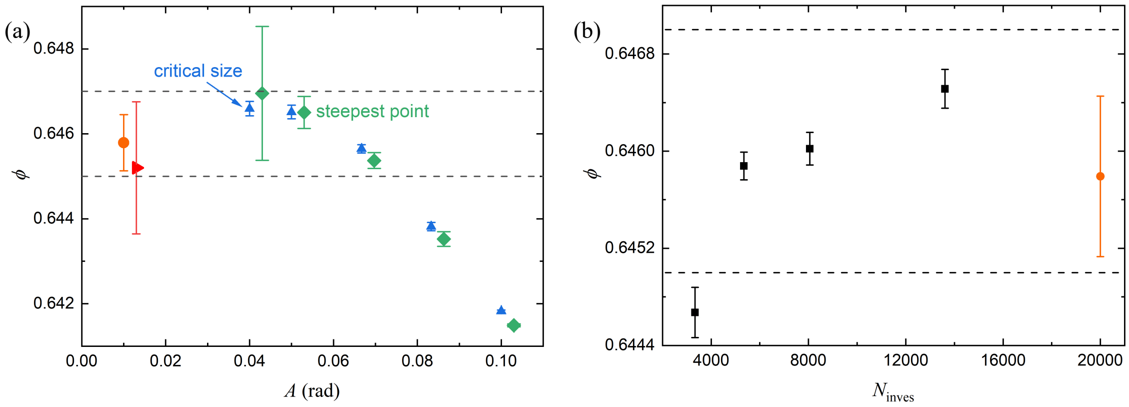


FIG. S7. (a) The global packing fraction at the onset of crystallization estimated using two methods, 1) the packing fraction at which the largest crystallite reaches the critical cluster size (blue upward triangles) and 2) the packing fraction which the slope of the largest crystallite versus packing fraction is the largest (green diamonds), plotted versus amplitude $A$. We also show data from the experiments of Rietz et al. at $A = 0.01$ rad, obtained using methods 1 (orange circle) and 2 (rightward red triangle). The data for method 2 are shifted slightly in $A$. The error bars correspond to the standard error in the mean. The standard error of the experimental data is an estimate from simulations at $A = 0.05$ with the assumption that they have a similar standard deviation. (b) The global packing fraction $\phi$ at the onset of crystallization (using method 1) plotted as a function of the number of grains $N$ for the simulations at amplitude $A = 0.05$ rad (black squares). The experimental data at $A = 0.01$ rad is indicated by an orange circle. The dashed lines correspond to the value of $\phi = 0.646 \pm 0.001$.

### D. Cyclic shear without gravity

The results for the simulations of cyclic shear in the main text were carried out in the presence of gravity. In this section, we compare the results for the global packing fraction from simulations of cyclic shear with and without gravity. Compared to frictionless systems with gravity, similar results can be observed in frictionless systems without gravity, as shown in Fig. S8. It shows a similar packing fraction of about 0.646 at onset, while systems with and without gravity have a slight difference in the structural properties during the crystallization (see Fig. S8(b)). Generally, we find that gravity, friction, and energy conservation are not required to yield homogeneous crystallization. In contrast, crystallization can be achieved in cyclically driven, dissipative particulate systems with volume exclusion, system confinement, and small disturbances that allow grain rearrangements.

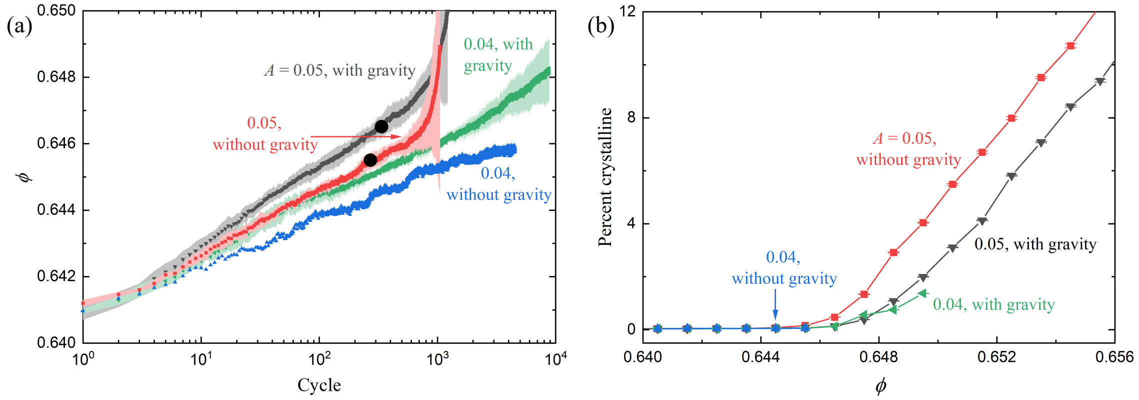


FIG. S8. (a) The global packing fraction $\phi$ plotted as a function of cycle number for simulations with and without gravity at shear amplitude $A = 0.04$ and 0.05 rad. The black point on each curve shows the characteristic packing fraction at crystallization onset. (b) The percentage of the grains that are crystalline plotted as a function of the global packing fraction for the same data in (a).

### E. Homogenous nucleation

In this section, we investigate the extent to which crystallites nucleate and grow in the central region of the simulation cell, not near the system walls. In Fig. S9, we show the probabilities $P(x)$ and $P(y)$ for the center of mass of crystallites (with sizes ranging from 15 to 25, which are close to the critical cluster size) to be located at horizontal position $x$ or vertical position $y$. We find that crystallites with sizes near the critical cluster size are roughly equally probable to occur over the accessible central regions of the system. In contrast, the probability of crystallites to occur near the top wall is larger than that near the bottom wall. The increased probability near the top wall may be caused by the pressure gradient in the system caused by the gravitational field, where grains near the top wall can rearrange more frequently. This effect decreases with increasing spring constant and vanishes in the $k \to \infty$ limit.

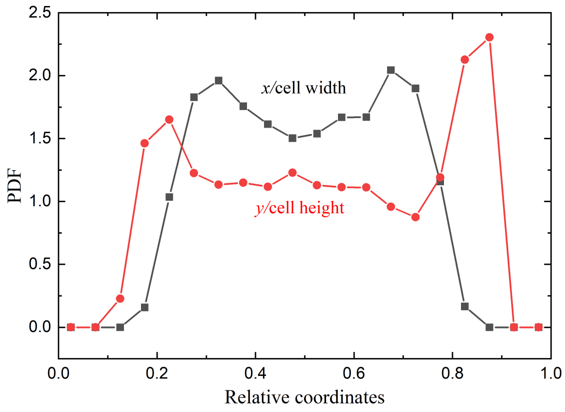


FIG. S9. The probability $P(x/w)$ (squares) and $P(y/h)$ that a crystallite has its center of mass at $x/w$ or at $y/h$, where $w = L + 2d$ is the width and $h = 1.675L$ is the height of the simulation cell (with its origin in the lower left corner in Fig. 1(a) in the main text). The data for the probability distributions are obtained from $10^4$ crystallites with sizes ranging from 15 to 25 grains from simulations with shear amplitude $A = 0.05, 0.0667, 0.0833$, and 0.1 rad and system size $N = 18200$.

*microwei.jin@gmail.com **shattuck@ccny.cuny.edu

[1] F. Rietz, C. Radin, H. Swinney and M. Schröter, Nucleation in sheared granular matter, *Phys. Rev. Lett.* 120, (2018) 055701
